# Supplementary material for: Coherent spin control of s-, p-, d- and f-electrons in a silicon quantum dot
Source: arXiv:1902.01550 ancillary file (2019-05-06)
Supplement: Supplementary file 1 [file supp.pdf]

# Supplementary Material: Coherent spin control of s-, p-, d- and f-electrons in a silicon quantum dot

R. C. C. Leon,[1,*] C. H. Yang,[1] J. C. C. Hwang,[1,†] J. Camirand Lemyre,[2] T. Tanttu,[1] W. Huang,[1] K. W. Chan,[1] K. Y. Tan,[3] F. E. Hudson,[1] K. M. Itoh,[4] A. Morello,[1] A. Laucht,[1] M. Pioro-Ladrière,[2,5] A. Saraiva,[1,‡] and A. S. Dzurak[1,§]

*[1]Centre for Quantum Computation and Communication Technology, School of Electrical Engineering and Telecommunications, The University of New South Wales, Sydney, NSW 2052, Australia.*

*[2]Institut Quantique et Département de Physique, Université de Sherbrooke, Sherbrooke, Québec J1K 2R1, Canada*

*[3]QCD Labs, COMP Centre of Excellence, Department of Applied Physics, Aalto University, 00076 AALTO, Finland*

*[4]School of Fundamental Science and Technology, Keio University, 3-14-1 Hiyoshi, Kohokuku, Yokohama 223-8522, Japan.*

*[5]Quantum Information Science Program, Canadian Institute for Advanced Research, Toronto, ON, M5G 1Z8, Canada*

## I. MICROMAGNET DESIGN

A layer of 460 $\mu$m long, 600 nm wide, 250 nm thick cobalt is deposited next to the Si-MOS structure shown in Fig. 1 of the main text. The cobalt width increases at regions further away from quantum dot, up to 80 $\mu$m, resulting in a trapezoidal prism structure. A 10 nm thick titanium layer is deposited before cobalt to ensure adhesion between $SiO_2$ and cobalt during deposition.

All experiments presented in the main text of the paper are carried at $B_0$ =1.4 T. Magnetic field simulations performed with Radia package of Mathematica (Supp. Fig. 1) indicate that the magnet produces a gradient of $\sim 1$ T/$\mu$m at the quantum dot location. This value can be considered constant in all experiments. Indeed, the quantization axis is well defined by the external field and the magnet is fully magnetized at such large field.

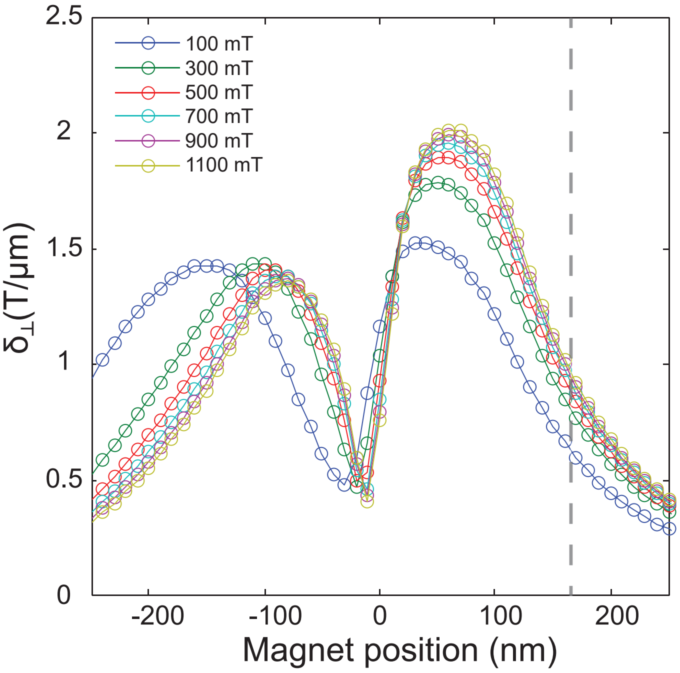


**Supplementary Figure 1**: **Magnetic field gradient produced by micromagnet.** Simulation of the transverse magnetic field gradient produced by the cobalt layer[1], at various applied external magnetic fields $B_0$. The grey dashed line indicates the position of the quantum dot.

## II. RABI FREQUENCIES AND POWER DEPENDENCE OF Q-FACTOR

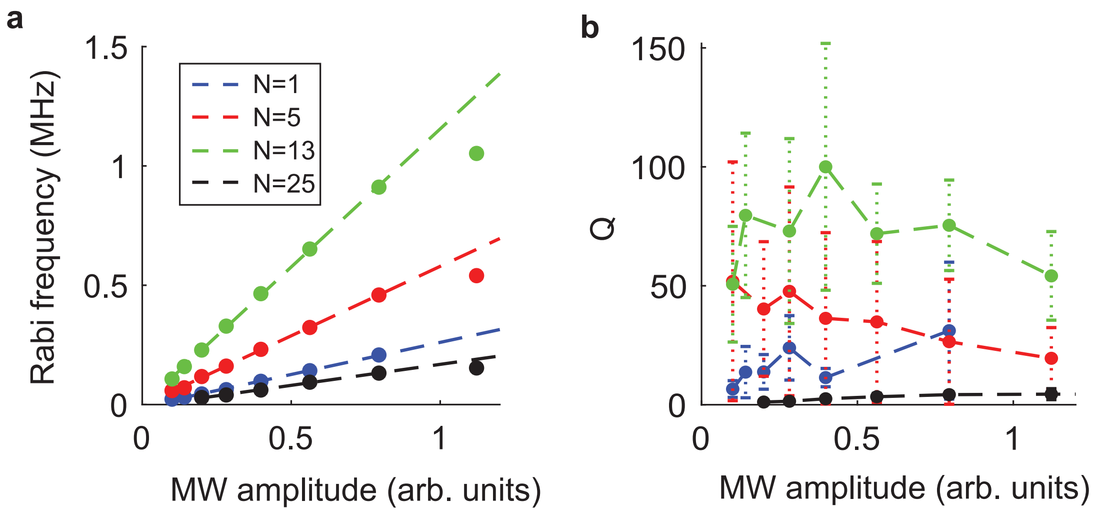


**Supplementary Figure 2**: **Microwave power dependence.** **(a)** Rabi frequency and **(b)** $Q$-factor as a function of applied microwave amplitude, at 1, 5, 13, 25 electrons configuration.

At s-, p-, d-, and f-electron occupations, Rabi frequencies increase linearly with microwave amplitude (Supp. Fig. 2a). As more electrons occupy the quantum dot, their wavefunction size increases and confinement energy decreases, hence leading to a higher effective oscillating magnetic field via EDSR[2]. Supp. Fig. 2a shows that the Rabi frequency increases as electron occupancies progress from s- to p- and d-electron. At the f-electron, other effects such as multiple relaxation hot spots prevent an optimal voltage configuration for the qubit, resulting in a inefficient Rabi drive.

One should note that the Dresselhaus spin-orbit coupling, which is dominant in Si, has very distinct impact on each valley state, which could potentially affect EDSR if it was driven by the material spin-orbit coupling[3,4]. Since our EDSR approach adopts an inhomogeneous magnetic field induced by a micromagnet, however, we expect that possible suppressions of spin-orbit effects by valley interference are overcome by the field gradient. In other words, the observed improvement of the Rabi oscillations is unlikely to largely stem from variations in the valley structure among shells.

Although variations of the $Q$-factor ($Q = T_2^{\mathrm{Rabi}}/T_\pi$) are observed for different electron occupancy, the MW amplitude dependence remains unclear. Previous work in Ref.5 has identified operation points where the applied microwave power maximizes the Q-factor. From values and error bars in Supp Fig. 2b, it is not possible to identify such optimal operation point.

## III. GATE VOLTAGE TUNING OF THE Q-FACTOR

As mentioned in the main text and Supp. Fig. 3a, qubit Rabi frequencies depend on the degree of confinement of the quantum dot, controlled by the gate voltages. Changing quantum dot confinement, on the other hand, may also increase its exposure to various noises. In Supp. Fig. 3b, $T_2^{\mathrm{Rabi}}$ varies up to an order of magnitude with changes in confinement level of the p-electron. As a result of Supp. Fig.3a and b, an optimal operation point is extracted with a maximum quality factor $Q$, as shown in Supp. Fig. 3c. Note that the d-electron qubit shares a similar behaviour as the p-electron, while the s-electron does not have any observable change in $Q$ due to the lack of excitation hotspots.

## IV. COHERENCE OF VARIOUS QUANTUM DOT FILLINGS

The coherence time $T_2^*$ is not significantly affected at different electron occupancies as seen in Table I. The main source of decoherence is electrical noise under magnetic field gradients[6]. Assuming a quantum dot radius of $a = 20$ nm, using equation (5) in Ref. 6, with in plane magnetic field gradient $\delta_{\parallel} = 0.8$ T/$\mu$m, we estimated $T_2^* \sim 50$ $\mu$s.

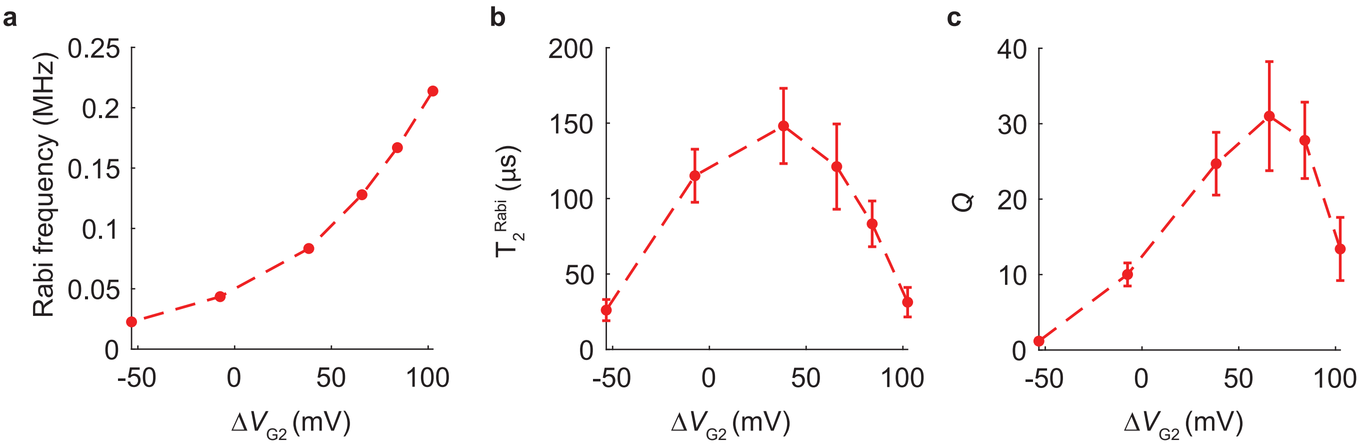


**Supplementary Figure 3**: **Confinement voltage dependent Q-factor.** **(a)** Rabi frequency, **(b)** $T_2^{Rabi}$ and **(c)** $Q$-factor as a function of change in gate voltage $\Delta V_{\rm G1}$ and $\Delta V_{\rm G2}$, following the dashed line in Fig. 3c of main text, at 5 electrons configuration.

Study in Ref. 7 reveals that decoherence due to 800ppm residual silicon-29 nuclei in an isotopically purified silicon wafer sets $T_2^*$ to 10-100 $\mu$s, meaning it can possibly be a contributing factor of decoherence.

Again, in Table I, $T_2^{\rm Hahn}$ of all electron occupancies are within an order of magnitude, with $T_2^{\rm Hahn}$ of $N$ =1 larger than $N = 5$ and 13 by a factor of 3. The larger coupling to charge noise could result in this lesser effect of the Hahn echo sequence. Interestingly, refocusing using Hahn echo is more beneficial to $N = 13$ than 5, possibly due to the differences between p-orbitals and d-orbitals. This is supported by a higher quality factor in $N = 13$ of Fig. 2b, where high frequency noises are filtered. On the other hand, the lower overall noise level in $T_2^*$ data at $N = 5$ than 13 agrees with the higher fidelity of the Clifford gates.

| Number of electrons | $T_2{}^*$ ($\mu$s) | $T_2^{\rm Hahn}$ ($\mu$s) |
|---|---|---|
| 1 | 18.1 | 68.5 |
| 5 | 15.7 | 21.6 |
| 13 | 7.75 | 28.9 |

TABLE I: Decoherence time of qubits at various electron occupancies.


* r.leon@student.unsw.edu.au
† Current address: Research and Prototype Foundry, The University of Sydney, Sydney, NSW 2006, Australia.
‡ a.saraiva@unsw.edu.au
§ a.dzurak@unsw.edu.au



[1] Wolfram Research, I. Mathematica (2018).

[2] Pioro-Ladrière, M. *et al.* Electrically driven single-electron spin resonance in a slanting Zeeman field. *Nature Physics* **4**, 776–779 (2008). URL http://www.nature.com/doifinder/10.1038/nphys1053{%}5Cnhttp://dx.doi.org/10.1038/nphys1053http://www.nature.com/articles/nphys1053. 0805.1083.

[3] Nowack, K. C., Koppens, F. H. L., Nazarov, Y. V. & Vandersypen, L. M. K. Coherent control of a single electron spin with electric fields. *Science (New York, N.Y.)* **318**, 1430–3 (2007). URL http://www.ncbi.nlm.nih.gov/pubmed/17975030.

[4] Corna, A. *et al.* Electrically driven electron spin resonance mediated by spin-valley-orbit coupling in a silicon quantum dot. *npj Quantum Information* **4**, 6 (2018). URL http://www.nature.com/articles/s41534-018-0059-1.

[5] Takeda, K. *et al.* A fault-tolerant addressable spin qubit in a natural silicon quantum dot. *Science Advances* **2**, e1600694 (2016). URL http://advances.sciencemag.org/lookup/doi/10.1126/sciadv.1600694.

[6] Kha, A., Joynt, R. & Culcer, D. Do micromagnets expose spin qubits to charge and Johnson noise? *Applied Physics Letters* **107**, 172101 (2015). URL http://aip.scitation.org/doi/10.1063/1.4934693.

[7] Zhao, R. *et al.* Coherent single-spin control with high-fidelity singlet-triplet readout in silicon. Tech. Rep. (2019). URL https://arxiv.org/pdf/1812.08347.pdf. 1812.08347v4.
